# Supplementary material for: Enhancing Semantic Fidelity in Text-to-Image Synthesis: Attention Regulation in Diffusion Models
Source: arXiv:2403.06381 source file (2024-03-11)
Supplement: Supplementary file 1 [file 6_appendix.tex]

\appendix
\section{Appendix}

\subsection{More Attention Statistics} \label{appx:more_attention_stats}

In this section, we provide a set of examples that illustrates the relationship between the distribution of the values of the attention weights and the semantic accuracy of the images generated by the model. 
The experiment setup is identical to that in Section 3 except for the selection of diffusion step and cross-attention layer. In this setup, we chose to plot the maximum value of each attention head in the first up-sampling layer at the final diffusion step. From Figure~\ref{fig:more_attn_plots_1} and Figure~\ref{fig:more_attn_plots_2}, we observe a positive relationship between the manifestation of a token in the generated image and the values of its attention weight. To illustrate, consider the first row of Figure~\ref{fig:more_attn_plots_1}. The attention values of the token "camera" is suppressed in the first four images (from the left), which corresponds to the absence of the camera in the generated image. However, in the final image in the first row, the attention values of the token "camera" is significantly higher, which corresponds to the presence of a camera in the generated image.

\begin{figure*}[t]
    \centering
    \includegraphics[width=\textwidth]{figs/more_attn_plots_1.png}
    \caption{\textbf{Generated Images and their Corresponding Attention Plots.} In the first row, the camera appears only when the attention values of the "camera" token match that of the "artichoke" token. In the second row, the apple appears only when the attention values of the "apple" token match that of the "leopard" token. In the third row, the attention values of the "glasses" token is significantly lower than the "chameleon" token, which corresponds to the absence of glasses in the generated images.}
    \label{fig:more_attn_plots_1}
\end{figure*}

\begin{figure*}[t]
    \centering
    \includegraphics[width=\textwidth]{figs/more_attn_plots_2.png}
    \caption{\textbf{Generated Images and their Corresponding Attention Plots.} In the first row, the attention values of the "rifle" token is significantly lower than the "owl" token, which corresponds to the absence of rifle in the generated images. In the second row, the sofa appears when the attention values of the "sofa" token follows a similar distribution as that of the "owl" token. In the third row, the apple appears only when the attention values of the "apple" token match that of the "dragonfly" token.}
    \label{fig:more_attn_plots_2}
\end{figure*}

\subsection{More Evaluation Metrics on Different Diffusion Models} \label{appx:more_evaluation_metrics}

\subsection{Experiment on Guidance Scale}\label{appx:guidance_scale}
\todo{add}

\subsection{More Visual Comparisons of Images} \label{appx:more_visual_comparison}

In this section, we provide more visual comparisons of generated images between the original Stable Diffusion, Attention Regulation and Attend and Excite methods. Figure~\ref{fig:more_visual_comparison} showcases an uncurated set of 3 images per prompt across 10 prompts covering multiple settings and objects. All images are generated with seed $42$ and our method uses the hyperparameter $\kappa$ set to 0.5. 

\begin{figure*}[t]
    \centering
    \includegraphics[width=\textwidth]{figs/img_comparison.png}
    \caption{\textbf{More Visual Comparison of Images.} We find that our method not only enhances the semantic fidelity of the generated images but also does so in a subtle manner where edits are done \textit{locally} thus preserving the overall structure of the images.}
    \label{fig:more_visual_comparison}
\end{figure*}

\subsection{More Ablation Results}\label{appx:more_ablation_results}
