# Supplementary material for: Enhancing Semantic Fidelity in Text-to-Image Synthesis: Attention Regulation in Diffusion Models
Source: arXiv:2403.06381 source file (2024-03-11)
Supplement: Supplementary file 3 [file 7_appendix_old.tex]

\section{Appendix}

\subsection{More Attention Statistics} \label{appx: more_attention_stats}

In this section, we provide a set of examples that illustrates the relationship between the distribution of the values of the attention weights and the semantic accuracy of the images generated by the model. 
The experiment setup is identical to that in Section 3 except for the selection of diffusion step and cross-attention layer. In this setup, we chose to plot the maximum value of each attention head in the first up-sampling layer at the final diffusion step. From Figure~\ref{fig:more_attn_plots_1} and Figure~\ref{fig:more_attn_plots_2}, we observe a positive relationship between the manifestation of a token in the generated image and the values of its attention weight. To illustrate, consider the first row of Figure~\ref{fig:more_attn_plots_1}. The attention values of the token "camera" is suppressed in the first four images (from the left), which corresponds to the absence of the camera in the generated image. However, in the final image in the first row, the attention values of the token "camera" is significantly higher, which corresponds to the presence of a camera in the generated image.

\begin{figure*}[t]
    \centering
    \includegraphics[width=\textwidth]{figs/more_attn_plots_1.png}
    \caption{\textbf{Generated Images and their Corresponding Attention Plots.} In the first row, the camera appears only when the attention values of the "camera" token match that of the "artichoke" token. In the second row, the apple appears only when the attention values of the "apple" token match that of the "leopard" token. In the third row, the attention values of the "glasses" token is significantly lower than the "chameleon" token, which corresponds to the absence of glasses in the generated images.}
    \label{fig:more_attn_plots_1}
\end{figure*}

\begin{figure*}[t]
    \centering
    \includegraphics[width=\textwidth]{figs/more_attn_plots_2.png}
    \caption{\textbf{Generated Images and their Corresponding Attention Plots.} In the first row, the attention values of the "rifle" token is significantly lower than the "owl" token, which corresponds to the absence of rifle in the generated images. In the second row, the sofa appears when the attention values of the "sofa" token follows a similar distribution as that of the "owl" token. In the third row, the apple appears only when the attention values of the "apple" token match that of the "dragonfly" token.}
    \label{fig:more_attn_plots_2}
\end{figure*}

\subsection{Bounds on Attention Value after Attention Regulation} \label{appx: bounds_on_attention_regulation}
In this section, we provide a bound on the value of the attention weights after attention regulation. We then use the proven results to provide an explanation of the effectiveness of our methods. We shall follow the notation used in Section 4.1 and 4.2.
\paragraph{Property 1} $\max(A_{i, t}(1 - \Gamma[t])) = \mathcal{I}_{avg}.$ \\
\quad \\
\textit{Proof.} 
\begin{align*}
    \max(A_{i, t}(1 - \Gamma[t])) &= \max(A_{i, t}) \times (1 - \Gamma[t]) \\
    &= I_{t} \left( \frac{\mathcal{I}_{avg}}{I_t} \right) \\
    &= \mathcal{I}_{avg} 
\end{align*}
\begin{flushright}
    $\square$
\end{flushright}

\paragraph{Property 2} Let $M = \max \mathcal{I}$, $I_{EOS} = \max(A_{i, EOS})$, $I_{p} = \max(A_{i, p})$ and 
$$\delta = \max\{I - \mathcal{I}_{avg} \ | \ I \in \mathcal{I} \setminus \{M\}\} + I_p.$$ 
Let $A'_1, A'_2, \dots, A'_n$ denote the attention weights for each token after attention regulation and let $M' = \max\{\max(A'_k) \ | \ 1 \leq k \leq n\}.$
Then, $$M' \leq \max\{\tau(\mathcal{I}_{avg} + \delta), I_l + \kappa I_{EOS}) \}.$$
\textit{Proof.} If $M \leq \tau(\mathcal{I}_{avg} + \delta) - \tau I_p$, by definition, the attention of the dominating token is not decreased. However, the attention of the least effective token is still enhanced. As such, we have 
\begin{align*}
    M' &\leq \max\{M, I_l + \kappa I_{EOS}\} \\
        &\leq \max\{\tau(\mathcal{I}_{avg} + \delta), I_l + \kappa I_{EOS}\}.
\end{align*}
If $M > \tau(\mathcal{I}_{avg} + \delta) - \tau I_p$, the attention value of the dominating token is decreased and by Property 1, we have $A'_t = \mathcal{I}_{avg} + \Gamma[t]I_{p} \leq \tau(\mathcal{I}_{avg} + \delta)$. Similarly, the attention of the least effective token is enhanced. As such, 
\begin{align*}
    M' &\leq \max\{\tau(\mathcal{I}_{avg} + \delta), I_l + \kappa I_{EOS}\}.
\end{align*}
\begin{flushright}
    $\square$
\end{flushright}

\paragraph{Remark} Notice that bound is independent of the attention values of the dominating token before attention regulation. 
The bound achieved provides an explanation for the effectiveness of our methods. In our experiment setup, we set $\tau = 1.1$, while $\kappa$ varies. Consider the case when $\kappa = 0$. 
This implies that $M' \leq 1.1(\mathcal{I}_{avg} + \delta)$. If $\delta$ is sufficiently small, then $M'$ would only be slightly more than $10\%$ larger than $\mathcal{I}_{avg}$. 
This suggests that the maximum values of the attention weights for each token are rather close, thus achieving a more balanced representation of the tokens. 
When $\kappa$ increases, the balanced representation of tokens is still maintained even though the maximum attention, $M'$, is deviating further from $\mathcal{I}_{avg}$. 
This is due to the summarizing property of the EOS token and the fact that it is added to the least effective token. 
The summarizing property maintains the balanced representation of tokens while the addition to the least effective token ensures that no important information is lost by modifying its attention weights as it had an extremely low contribution to begin with.

\subsection{Lang-SAM + CLIP Evaluation Details} \label{appx: langSAM_eval_details}

\paragraph{Formal Description} This evaluation comprises of two stages, namely the image segmentation stage and the text-image comparison stage. 
Given an image $\mathcal{I}$ and a string representation of a target object $\mathcal{O}$, we aim to construct a scoring function that evaluates the semantic accuracy between the image and the target object. We shall denote this scoring function as $\psi(\cdot, \cdot)$.
Firstly, we utilize the Lang-SAM model, $\phi(\cdot, \cdot)$, to acquire the set of bounding boxes of the region of the image that contains the target object, given by $\phi(\mathcal{I}, \mathcal{O})$. 
Then, for each bounding box, $B$, in $\phi(\mathcal{I}, \mathcal{O})$, we utilize the CLIP model, $\zeta(\cdot, \cdot)$, to compute the image-text similarity score, given by $\zeta(\mathcal{I}[B], \mathcal{O})$, where $\mathcal{I}[B]$ refers to the region of image $\mathcal{I}$ contained within the bounding box $B$. 
Finally, we have
$$ \psi(\mathcal{I}, \mathcal{O}) = \max_{B \in \phi(\mathcal{I}, \mathcal{O})} \zeta(\mathcal{I}[B], \mathcal{O}). $$
Note that $\psi(\mathcal{I}, \mathcal{O})$ is defined to be $0$ if $\phi(\mathcal{I}, \mathcal{O}) = \emptyset$.

\paragraph{Remark} We shall clarify the difference between our Lang-SAM + CLIP evaluation and the previously used CLIP evaluation. 
The distinction is presented in the following setup. 
Consider an image $\mathcal{I}$ and a string representation of the prompt $\mathcal{P}$ which contains two target objects, $\mathcal{O}_1$ and $\mathcal{O}_2$. 
The score of the image given by our Lang-SAM + CLIP evaluation is $\min \{ \psi(\mathcal{I}, \mathcal{O}_1), \psi(\mathcal{I}, \mathcal{O}_2) \}$, whereas the score of the given by CLIP evaluation is $\zeta(\mathcal{I}, \mathcal{P})$. 
While both approaches utilizes the CLIP model, our approach is likely to be more accurate as our inputs given to the CLIP model, $\mathcal{I}[B], \mathcal{O}_1, \mathcal{O}_2$, are more specific as $\mathcal{I}[B] \subseteq \mathcal{I}$ and $\mathcal{O}_1, \mathcal{O}_2 \subseteq \mathcal{P}$.

\subsection{More Visual Comparisons of Images} \label{appx: more_visual_comparison}

In this section, we provide more visual comparisons of generated images between the original Stable Diffusion, Attention Regulation and Attend and Excite methods. Figure~\ref{fig:more_visual_comparison} showcases an uncurated set of 3 images per prompt across 10 prompts covering multiple settings and objects. All images are generated with seed $42$ and our method uses the hyperparameter $\kappa$ set to 0.5. More details on $\kappa$ can be found in Section~\ref{appx: kappa_ablation}.

\begin{figure*}[t]
    \centering
    \includegraphics[width=\textwidth]{figs/img_comparison.png}
    \caption{\textbf{More Visual Comparison of Images.} We find that our method not only enhances the semantic fidelity of the generated images but also does so in a subtle manner where edits are done \textit{locally} thus preserving the overall structure of the images.}
    \label{fig:more_visual_comparison}
\end{figure*}



\subsection{Ablation Study on $\kappa$} \label{appx: kappa_ablation}

In this section, we illustrate the effect varying the value of the hyperparameter $\kappa$. 
From the first three rows of Figure~\ref{fig:kappa_abaltion}, we can observe that increasing the $\kappa$ value can result in more semantically accurate images. 
However, from the last two rows, we observe that for cases where attention regulation with $\kappa = 0$ is already sufficient to generate semantically accurate images, increasing the $\kappa$ value can result in slight deterioration of the image quality. 
As such, to increase the quality of the images, for a specific prompt and latent, we recommend that the $\kappa$ is gradually increased to achieve a balance between semantic accuracy and image quality.

\begin{figure*}[t]
    \centering
    \includegraphics[width=\textwidth]{figs/kappa_ablation.png}
    \caption{\textbf{Effects of Varying Hyperparameter $\kappa$.} From left to right, the $\kappa$ value varies from $0$ to $1$, at equal intervals. The semantic accuracy of the images increased as the $\kappa$ value increased in the first three rows, while the semantic accuracy remained the same for the last two rows. This is due to the fact that a semantically accurate image is already generated when $\kappa = 0$ for the last two rows. As such, it is unnecessary to increase the $\kappa$ value to increase the amount of summary information. As shown in the last two rows, unnecessarily increasing the $\kappa$ value can result in quality degradation.}
    \label{fig:kappa_abaltion}
\end{figure*}

\subsection{More Results on Layer Ablation Study} \label{appx: more_layer_ablation}

In this section, we further illustrate the effect varying the number of cross-attention layers that are edited. 
From Figure~\ref{fig:more_layer_ablation}, we observe similar results to Figure~\ref{fig:ablation_layers_sample}, where the increase in effectiveness of attention regulation saturates as the number of cross-attention layers that are edited increases. 

\begin{figure*}[t]
    \centering
    \includegraphics[width=\textwidth]{figs/more_layer_ablation.png}
    \caption{\textbf{Effects of Varying the Number of Edit Layers.} From left to right, the number of edit layers vary across $0$, $2$, $4$, $6$ and $7$. Similar to results shown in Figure~\ref{fig:ablation_layers_sample}, semantic accuracy of the generated images increases significantly when the number of edit layers are small. However, as the number of edit layers increase, the semantic accuracy saturates and has minimal effect on the image generated.}
    \label{fig:more_layer_ablation}
\end{figure*}

\subsection{More Results on Step Ablation} \label{appx: more_step_ablation}

In this section, we further illustrate the effect increasing the terminal step with attention regulation. 
From Figure~\ref{fig:more_step_ablation}, we observe similar results to Figure~\ref{fig:step_ablation}, where the increase in effectiveness of attention regulation saturates as the terminal step increases. 

\begin{figure*}[t]
    \centering
    \includegraphics[width=\textwidth]{figs/more_steps_ablation.png}
    \caption{\textbf{Effects of Varying the Number of Edit Steps.} From left to right, the terminal steps vary from $0$ to $40$ at equal intervals. Similar to results shown in Figure~\ref{fig:ablation_steps_sample}, semantic accuracy of the generated images increases significantly when the number of edit steps are small. However, as the number of edit steps increase, the semantic accuracy saturates and has minimal effect on the image generated.}
    \label{fig:more_step_ablation}
\end{figure*}

\subsection{More Examples on Style Transfer} \label{appx: more_style_transfer}
In this section, we give more examples and illustrations of style transfer applications like the one seen in Figure~\ref{fig:style_transfer_demo}. The first row of every prompt uses the generation without attention regulation while the second uses our method with attention regulation. Examples can be seen at Figure~\ref{fig:styletransfer1} and Figure~\ref{fig:styletransfer2}.

\begin{figure*}[t]
    \centering
    \includegraphics[width=\textwidth]{figs/styletransfer1.png}
    \caption{\textbf{Examples of Style transfer.} Successful transfer of art/artist styles onto subject can be achieved with our method as compared to having no attention regulation.}
    \label{fig:styletransfer1}
\end{figure*}

\begin{figure*}[t]
    \centering
    \includegraphics[width=0.8\textwidth]{figs/styletransfer2.png}
    \caption{\textbf{Examples of Style transfer.} Examples of style transfer on single subject (Mona Lisa) across different art styles.}
    \label{fig:styletransfer2}
\end{figure*}

\subsection{More Examples on Copyright} \label{appx: more_copyright}
In this section, we provide more examples and illustrations of copyright protection applications. The images generated in the first rows of every prompt uses the generation without attention regulation while the second uses our method with attention regulation. Examples can be seen at Figure~\ref{fig:more_copyright_1} and Figure~\ref{fig:more_copyright_2}.

\begin{figure*}[t]
    \centering
    \includegraphics[width=\textwidth]{figs/more_copyright_1.png}
    \caption{\textbf{Examples of Copyright Protection.} In situations where the original SD 2 model overfits to copyrighted features, like the "S" logo of Superman and the Captain America uniform, attention regulation reduces the attention on these concepts. This enables the generation of images with significantly less, or zero in many cases, copyrighted features, while preserving the stylistic similarities.}
    \label{fig:more_copyright_1}
\end{figure*}

\begin{figure*}[t]
    \centering
    \includegraphics[width=\textwidth]{figs/more_copyright_2.png}
    \caption{\textbf{Examples of Copyright Protection.} Through reducing the attention on copyrighted features via attention regulation, the regulated model is able to generate new logos that frequently contain stylistic similarities to the original without generating the copyrighted features.}
    \label{fig:more_copyright_2}
\end{figure*}
